# Supplementary material for: Personalization of Web Search During the 2020 US Elections
Source: arXiv:2209.14000 source file (2022-09-28)
Supplement: Supplementary file 1 [file tab_SM_serp_similarity.tex]

% Table created by stargazer v.5.2.2 by Marek Hlavac, Harvard University. E-mail: hlavac at fas.harvard.edu
% Date and time: Wed, Jun 09, 2021 - 10:17:27 PM
\begin{table}[!htb] \centering 
  \caption{Differences in search results pages} 
  \label{tab:SM_serp_similarity} 
\small 
\begin{tabular}{@{\extracolsep{5pt}}lcccc} 
\\[-1.8ex]\hline 
\hline \\[-1.8ex] 
 & \multicolumn{4}{c}{\emph{Dependent variable:} SERP similarity} \\ 
\cline{2-5} 
\\[-1.8ex] & \multicolumn{2}{c}{Jaccard} & \multicolumn{2}{c}{RBO} \\ 
\\[-1.8ex] & (1) & (2) & (3) & (4)\\ 
\hline \\[-1.8ex] 
 Same ideology & $-$0.0002 & 0.0001 & $-$0.0002 & $-$0.0001 \\ 
  & (0.001) & (0.001) & (0.001) & (0.0004) \\ 
  & & & & \\ 
 Same city & 0.011$^{**}$ & 0.010$^{***}$ & 0.010$^{**}$ & 0.007$^{***}$ \\ 
  & (0.005) & (0.002) & (0.005) & (0.001) \\ 
  & & & & \\ 
 Same browser language & 0.055$^{***}$ & 0.037$^{**}$ & 0.041$^{***}$ & 0.018$^{*}$ \\ 
  & (0.010) & (0.017) & (0.009) & (0.010) \\ 
  & & & & \\ 
 Time difference (days) & $-$0.006$^{***}$ & $-$0.007$^{***}$ & $-$0.005$^{***}$ & $-$0.005$^{***}$ \\ 
  & (0.001) & (0.002) & (0.001) & (0.001) \\ 
  & & & & \\ 
\hline \\[-1.8ex] 
Search term FE & X & X & X & X \\ 
Sample & Organic results & Topstories & Organic results & Topstories \\ 
Observations & 8,956,604 & 1,673,737 & 8,956,604 & 1,673,737 \\ 
R$^{2}$ & 0.453 & 0.308 & 0.542 & 0.337 \\ 
Adjusted R$^{2}$ & 0.453 & 0.308 & 0.542 & 0.337 \\ 
\hline 
\hline \\[-1.8ex] 
\multicolumn{5}{p{12cm}}{\emph{Notes:} OLS regressions with robust standard errors two-way clustered by search term and synthetic user pair. The unit of observation is search term-user pair. The dependent variable is the Rank-Biased Overlap
                 computed from different SERP parts (organic search results, top stories, ads) of SERPs presented to a user $i$ and a user $j$ when using the same search term. 
                    The explanatory variable \emph{`Same ideology'} is equal to 1 if users i and j have the same political ideology (either D, R, or apolitical) and 0 otherwise. 
                    The explanatory variable \emph{`Same city'} is equal to 1 if users i and j are located in the same city and 0 otherwise. 
                    The explanatory variable \emph{`Same browser language'} is equal to 1 if users i and j use the same language setting in their web browser and 0 otherwise. 
                    The explanatory variable \emph{`Time difference (days)'} is the absolute time difference between the searches of i and j, measured in (fraction of) days. Since some search terms have been used on several days 
                    throughout the entire duration of the experiment and since we are comparing all searches of all bots using the same search term, the difference can be sevaral days in these comparisons.
                    If a bot pair issued the search on the same date in the same city, the searches were also usually issued within minutes of the same time of the day.
                    In all specifications we account for search term fixed effects (as some user pairs might have used the same search term more than once). The statistical significance of coefficient estimates is indicated as follows: $^{*}$p$<$0.1; $^{**}$p$<$0.05; $^{***}$p$<$0.01.} \\ 
\end{tabular} 
\end{table}
